# Supplementary material for: On String Vacua without Supersymmetry: brane dynamics, bubbles and holography
Source: arXiv:2010.00628 source file (2021-07-16)
Supplement: Supplementary file 1 [file Appendix_integral.tex]

% Appendix Template

\chapter{\textcolor{mdtRed}{\textbf{Holographic integral geometry: a brief review}}} % Main appendix title

\label{sec:igappendix} % Change X to a consecutive letter; for referencing this appendix elsewhere, use \ref{AppendixX}
\thispagestyle{empty}
\numberwithin{equation}{chapter}
In this section we review the basics of Integral Geometry in the hyperbolic plane, since it concerns the specific case of $\ads_3/\cft_2$. A more comprehensive review can be found in~\cite{Czech2015}.

In this context the main object of interest is the topological space of ``lines'' in an asymptotically $\mathbb{H}^2$ bulk time-slice, namely the set of extremal curves between two boundary points, which constitutes the kinematic space $\mathcal{K}_2$. This is a two-dimensional surface that has a natural symplectic (or equivalently Lorentzian) structure, the \textit{Crofton form}, induced from the (finite part of the) length $\mathcal{L}$ of curves in $\mathcal{K}_2$ via
\begin{equation}
     \omega(u,v) \equiv \pdv{\mathcal{L}(u,v)}{u}{v} \, du \wedge dv  = 4G_3 \pdv{S_\text{ent}(u,v)}{u}{v} \, du \wedge dv \, ,
\end{equation}
where $G_3$ is the three-dimensional Newton constant and $u$, $v$ are angular coordinates for the endpoints on the $\mathbb{S}^1$ boundary. The last equality holds assuming the Ryu-Takayanagi formula, and the Crofton form $\omega$ also affords an information-theoretic interpretation in terms of mutual conditional information~\cite{Czech2015}. In addition, one may define an induced Lorentzian metric
\begin{equation}\label{eq:kinetic_metric}
    ds_{\mathcal{K}_2}^2 \equiv \pdv{\mathcal{L}}{u}{v} \, du \, dv \, .
\end{equation}

In the case of an $\ads_3$ vacuum, indeed composed of $\mathbb{H}^2$ slices, the Crofton form reduces to
\begin{equation}
    \omega_0(u,v) = \frac{L}{2\sin^2(\frac{u-v}{2})} \, du \wedge dv \, ,
\end{equation}
which is actually the only $SO(1,2)$-invariant $2$-form on kinematic space up to rescalings. Indeed, $\omega_0 = \vol_{\ds_2}$ is the volume form on two-dimensional de Sitter spacetime\footnote{Some intuition on this obtains embedding $\mathbb{H}^2$ in $\mathbb{R}^{1,2}$ as a two-sheeted hyperboloid, where hyperbolic lines arise from intersection with time-like planes through the origin. Such planes are in a one-to-one correspondence with their unit space-like normal vectors, which lie in the $\ds_2$ one-sheeted hyperboloid.}, and $\mathcal{K}^{(0)}_{2}$ is naturally endowed with the Lorentzian structure of $\ds_2$.

For a general deformed metric, which is still asymptotically $\mathbb{H}_-^2$ in any constant-time slice, one finds that the corresponding kinematic space is $\ds_2^-$ asymptotically, in the limit of large (absolute) de Sitter time, while the central region of small $\abs{t}$ is modified. In the kinematic picture, which acts as an intermediary, the vacuum bubble originates as a perturbation in $\omega$ from $\vol_{\ds_2}$, which is localised around the throat and expands symmetrically in the $\ds_2$ past and future as bulk time progresses, establishing in its interior the \textit{new} $\ds_2^+$, of different radius, associated with $\mathbb{H}^2_+$.

The relevance of this construction comes from a classical theorem of Crofton, which states that the length of any (not necessarily geodesic) bulk curve $\gamma$ can be computed in terms of an area in $\mathcal{K}_2$, namely
\begin{equation}\label{eq:crotfon_thm}
    \mathcal{L}[\gamma] = \frac{1}{4} \int_{\kappa \in \mathcal{K}_2} \omega(\kappa)\, n_{\gamma,\kappa}
\end{equation}
where $n_{\gamma,\kappa}$ is the (signed) intersection number of the curves $\gamma$ and $\kappa$. Hence, excluding shadow effects~\cite{Hubeny:2013gta, Freivogel:2014lja}, which are absent in this case, the bulk geometry is completely reconstructable from the Crofton form, which therefore provides an amount of information equivalent to the full entanglement entropy.
