# Supplementary material for: On String Vacua without Supersymmetry: brane dynamics, bubbles and holography
Source: arXiv:2010.00628 source file (2021-07-16)
Supplement: Supplementary file 2 [file AppendixTemplate.tex]

% Appendix Template

\chapter{Appendix Title Here} % Main appendix title

\label{AppendixX} % Change X to a consecutive letter; for referencing this appendix elsewhere, use \ref{AppendixX}
\thispagestyle{empty}

Write your Appendix content here.
